# Supplementary material for: Functional Regression on Manifold with Contamination
Source: arXiv:1704.03005 source file (2020-06-05)
Supplement: Supplementary file 1 [file supplementary.pdf]

# Supplementary Material for “Functional Regression on Manifold with Contamination”

Zhenhua Lin\*

Fang Yao\*<sup>†</sup>

## S.1 Auxiliary Results

For convenience, in the sequel we might simplify  $\mathcal{L}^2(D)$  by  $\mathcal{L}^2$ , and use  $\|\cdot\|$  to denote the norm  $\|\cdot\|_{\mathcal{L}^2}$  when no confusion arises.

**Proposition S.1.** *The embedding  $X$  defined in Example 1 is an isometric embedding. Moreover, there is no finite-dimensional linear subspace of  $\mathcal{L}^2(D)$  that fully contains the image  $X(S^1)$ .*

PROOF. Let  $V = \{(\cos \omega, \sin \omega) : \omega \in (a, b)\}$  be a local neighborhood of  $v$ , and let  $\psi(v) = \omega \in (a, b)$  for  $v = (v_1, v_2) = (\cos \omega, \sin \omega) \in V$ . Then  $\psi$  is a chart of  $S^1$ . Let  $U$  be open in  $\mathcal{L}^2$  such that  $X(v) \in U$ . Since  $\mathcal{L}^2$  is a linear space, the identity map  $\mathbf{I}$  serves as a chart. Let  $X_{U,V} : \psi(V) \rightarrow \mathcal{L}^2$  denote the map  $X \circ \psi^{-1}$ . Let  $\vartheta = \sqrt{C} \sum_k k^{-c+1} \{-\sin(k\omega)\phi_{2k-1} + \cos(k\omega)\phi_{2k}\}$ . It defines a linear

---

\*Department of Statistical Sciences, University of Toronto.

<sup>†</sup>Department of Probability and Statistics, Peking University. Email: fyao@utstat.toronto.edu

map from  $\mathbb{R}$  to  $\mathcal{L}^2$ , denoted by  $\Theta(t) = t\vartheta \in \mathcal{L}^2$ . Then,

$$\begin{aligned}
A(t) &\equiv t^{-2} \|X_{U,V}(\omega + t) - X_{U,V}(\omega) - \Theta(t)\|^2 \\
&= C \sum_{k=1}^{\infty} \left\{ \frac{k^{-c} \cos(k\omega + kt) - k^{-c} \cos(k\omega) + tk^{-c+1} \sin(k\omega)}{t} \right\}^2 + \\
&\quad C \sum_{k=1}^{\infty} \left\{ \frac{k^{-c} \sin(k\omega + kt) - k^{-c} \sin(k\omega) - tk^{-c+1} \cos(k\omega)}{t} \right\}^2 \\
&\equiv CB_1^2(t) + CB_2^2(t).
\end{aligned}$$

By Lipschitz property of the function

$$B_{1,k}(t) \equiv k^{-c} \cos(k\omega + kt) - k^{-c} \cos(k\omega) + tk^{-c+1} \sin(k\omega),$$

we conclude that  $|B_{1,k}(t)| \leq t \sup_t |B'_{1,k}(t)| \leq 2k^{-c+1}t$ . This implies that  $\sup_t B_1^2(t) \leq \sum_k 4k^{-2c+2} < \infty$ . By similar reasoning,  $\sup_t B_2^2(t) < \infty$  and hence  $\sup_t A(t) < \infty$ . We now apply Dominated Convergence Theorem to conclude that

$$\lim_{t \rightarrow 0} A(t) = C \lim_{t \rightarrow 0} \{B_1^2(t) + B_2^2(t)\} = C \sum_{k=1}^{\infty} \lim_{t \rightarrow 0} \left\{ \frac{B_{1,k}(t)}{t} \right\}^2 + C \sum_{k=1}^{\infty} \lim_{t \rightarrow 0} \left\{ \frac{B_{2,k}(t)}{t} \right\}^2 = 0.$$

By recalling that the tangent space  $T_{v_\omega} S^1$  at  $v_\omega$  is  $\mathbb{R}$  and the tangent space  $T_{X(v_\omega)} \mathcal{L}^2(D)$  at  $X(v_\omega)$  is  $\mathcal{L}^2(D)$ , the above shows that the differential map  $X_{*,v_\omega} : T_{v_\omega} S^1 \rightarrow T_{X(v_\omega)} \mathcal{L}^2(D)$  at  $v_\omega$  is given by the linear map  $\Theta$ , i.e.,

$$X_{*,v_\omega}(t) = \Theta(t) = t \sum_k \sqrt{C} k^{-c+1} \{-\sin(k\omega) \phi_{2k-1} + \cos(k\omega) \phi_{2k}\},$$

and the embedded tangent space at  $v_\omega$  is  $\text{span}\{-\sum_k k^{-c+1} \sin(k\omega) \phi_{2k-1} + \sum_k k^{-c+1} \cos(k\omega) \phi_{2k}\}$ . As this differential map is injective at all  $v \in S^1$ ,  $X$  is indeed an immersion. Since  $S^1$  is compact,  $X$

is also an embedding, and the image  $X(S^1)$  is a submanifold of manifold in  $\mathcal{L}^2(D)$ .

To show that  $X$  is isometric, note that the tangent space of  $S^1$  at  $v$  is the real line  $\mathbb{R}$ , equipped with the usual inner product  $\langle s, t \rangle = st$  for  $s, t \in \mathbb{R}$ . Let  $\langle\langle f_1, f_2 \rangle\rangle = \int_D f_1(t)f_2(t)dt$  for  $f_1, f_2 \in \mathcal{L}^2(D)$  denote the canonical inner product of  $\mathcal{L}^2(D)$ . Recalling the definition  $C = 1/\sum_{k=1}^{\infty} k^{-2c+2}$  in the example, we deduce that

$$\begin{aligned} \langle\langle X_{*,v\omega}(s), X_{*,v\omega}(t) \rangle\rangle &= \langle\langle \Theta(s), \Theta(t) \rangle\rangle = st \langle\langle \vartheta, \vartheta \rangle\rangle \\ &= Cst \sum_{k=1}^{\infty} \{k^{-2c+2} \sin^2(k\omega) + k^{-2c+2} \cos^2(k\omega)\} \\ &= Cst \sum_{k=1}^{\infty} k^{-2c+2} = st = \langle s, t \rangle, \end{aligned}$$

which shows that  $X$  is isometric.

Finally, to show that there is no finite-dimensional linear subspace of  $\mathcal{L}^2(D)$  that fully contains  $X(S^1)$ , we take the strategy of “proof by contradiction” to assume that  $H$  is a finite-dimensional linear subspace of  $\mathcal{L}^2(D)$  such that  $X(S^1) \subset H$ . Since  $H$  is finite-dimensional, there exists  $0 \neq \varphi \in \mathcal{L}^2(D)$  such that  $\varphi \perp H$  and hence  $\varphi \perp X(S^1)$ , or more specifically,  $\langle\langle \varphi, x \rangle\rangle = 0$  for each  $x \in X(S^1)$ . As  $\phi_1, \phi_2, \dots$  form a complete orthonormal basis of  $\mathcal{L}^2(D)$ , we can find real numbers  $a_1, a_2, \dots$  such that  $\varphi = \sum_k (a_{2k-1}\phi_{2k-1} + a_{2k}\phi_{2k})$ . Then,  $\langle\langle \varphi, x \rangle\rangle = 0$  for each  $x \in X(S^1)$  is equivalent to  $\sum_k k^{-c} \{a_{2k-1} \cos(k\omega) + a_{2k} \sin(k\omega)\} = 0$  for all  $\omega$ . Since  $\cos(k\omega)$  and  $\sin(k\omega)$ , as functions of  $\omega$ , are orthogonal, it implies that  $a_{2k-1} = 0$  and  $a_{2k} = 0$  for all  $k$ , which indicates that  $\varphi = 0$ . However, by assumption,  $\varphi \neq 0$ , and we draw a contradiction.  $\square$

Next result asserts that the local neighborhood based on contaminated data  $\hat{X}_i$  is indeed close to that based on true  $X_i$  with large probability.

**Proposition S.2.** Define  $h_- = h_{pca} - n^{-(\beta+\varrho)/2}$  and  $h_+ = h_{pca} + n^{-(\beta+\varrho)/2}$ . Let  $Z_i = 1_{\{\hat{X}_i \in \mathbb{B}_{h_{pca}}^{\mathcal{L}^2}(x)\}}$ ,  $V_{i0} = 1_{\{X_i \in \mathbb{B}_{h_-}^{\mathcal{L}^2}(x)\}}$  and  $V_{i1} = 1_{\{X_i \in \mathbb{B}_{h_+}^{\mathcal{L}^2}(x)\}}$ . Under assumption (B3) in the paper, then  $\Pr(\forall i : V_{i0} \leq$

$Z_i \leq V_{i1}) \rightarrow 1, n \rightarrow \infty.$

Hence one can always obtain lower and upper bounds for quantities involving  $Z_i$  in terms of  $V_{i0}$  and  $V_{i1}$ , i.e., with large probability, it is equivalent to substitute  $Z_i$  with  $V_{i0}$  and  $V_{i1}$  in our analysis.

PROOF. We first bound the following event

$$\begin{aligned} \Pr(\forall i : Z_i \leq V_{i1}) &= \prod_{i=1}^n \{1 - \Pr(Z_i > V_{i1})\} = \{1 - \Pr(Z > V_1)\}^n \\ &= \{1 - \Pr(Z = 1, V_1 = 0)\}^n \geq \left\{1 - \Pr(\|\hat{X} - X\| \geq n^{-(\beta+\varrho)/2})\right\}^n \\ &\geq \left(1 - c_1^p n^{p(\beta+\varrho)/2} n^{-p\beta}\right)^n \geq \left(1 - c_1^p n^{-2}\right)^n \rightarrow 1, \end{aligned}$$

where  $c_1 > 0$  is some constant, and  $p > 0$  is a constant that is sufficiently large so that  $p(\beta - \varrho) \geq 4$ . Similarly, we can deduce that

$$\Pr(\forall i : V_{i0} \leq Z_i) \rightarrow 1,$$

and the conclusion  $\Pr(\forall i : V_{0i} \leq Z_i \leq V_{1i}) \rightarrow 1$  follows.  $\square$

## S.2 Technical Lemmas

Here we collect some technical lemmas that will be used in the proofs of Theorems in the paper. The lemma below is used to establish Proposition 1. The proof of the lemma depends on Lemma S.2 and S.3.

**Lemma S.1.** *Suppose  $h_0 \rightarrow 0$ , and  $mh_0 \rightarrow \infty$ . For any  $p \geq 1$ , assume  $\mathbf{E}|\zeta|^p < \infty$ . Under assumptions (A1)–(A3), for the estimate  $\hat{X}$  in (4) with a proper choice of  $\delta$ ,*

$$\{\mathbf{E}(\|\hat{X} - X\|_{\mathcal{L}^2}^p \mid X)\}^{1/p} = O\left(m^{-1/2} h_0^{-1/2}\right) \left\{\sup_t |X(t)| + L_X\right\} + O(h_0^\nu) L_X, \quad (\text{S.1})$$

where  $O(\cdot)$  does not depend on  $X$ .

PROOF. In order to reduce notations, let  $h = h_0$ . Denoting  $\Delta = \delta 1_{|S_0 S_2 - S_1^2| < \delta}$  with  $\delta = m^{-2}$ , according to (4), we have

$$\hat{X}(t) - X(t) = \frac{S_2(R_0 - S_0 X)}{S_0 S_2 - S_1^2 + \Delta} - \frac{S_1(R_1 - S_1 X)}{S_0 S_2 - S_1^2 + \Delta} - \frac{\Delta X}{S_0 S_2 - S_1^2 + \Delta} \equiv I_1 + I_2 + I_3.$$

Therefore,

$$\|\hat{X} - X\|^p \leq c_p(\|I_1\|^p + \|I_2\|^p + \|I_3\|^p) \quad (\text{S.2})$$

for some constant  $c_p$  depending on  $p$  only.

For  $I_1$ , we have

$$\begin{aligned} \|I_1\|^p &= \left[ \int_D \left\{ \frac{S_2(R_0 - S_0 X)}{S_0 S_2 - S_1^2 + \Delta} \right\}^2 dt \right]^{p/2} \leq \left[ \int_D \{S_2(R_0 - S_0 X)\}^4 dt \int_D \left( \frac{1}{S_0 S_2 - S_1^2 + \Delta} \right)^4 dt \right]^{p/4} \\ &\leq \left\{ \int_D S_2^8 dt \int_D (R_0 - S_0 X)^8 dt \right\}^{p/8} \left\{ \int_D \left( \frac{1}{S_0 S_2 - S_1^2 + \Delta} \right)^4 dt \right\}^{p/4}. \end{aligned}$$

This also shows that, for  $p \geq 2$ ,

$$\begin{aligned} &\mathbf{E}(\|I_1\|^p \mid X) \\ &\leq \left( \mathbf{E} \left\{ \left[ \int_D S_2^8 dt \int_D (R_0 - S_0 X)^8 dt \right]^{p/4} \mid X \right\} \right)^{1/2} \left( \mathbf{E} \left\{ \left[ \int_D \left( \frac{1}{S_0 S_2 - S_1^2 + \Delta} \right)^4 dt \right]^{p/2} \mid X \right\} \right)^{1/2} \\ &\leq \left( \mathbf{E} \left[ \int_D S_2^{4p} dt \right] \mathbf{E} \left[ \int_D (R_0 - S_0 X)^{4p} dt \mid X \right] \right)^{1/4} \left( \mathbf{E} \left[ \int_D \left\{ \frac{1}{S_0 S_2 - S_1^2 + \Delta} \right\}^{2p} dt \right] \right)^{1/2} \\ &= \left\{ \int_D \mathbf{E}(S_2^{4p}) dt \right\}^{1/4} \left[ \int_D \mathbf{E}\{(R_0 - S_0 X)^{4p} \mid X\} dt \right]^{1/4} \left[ \int_D \mathbf{E} \left\{ \left( \frac{1}{S_0 S_2 - S_1^2 + \Delta} \right)^{2p} \right\} dt \right]^{1/2}. \quad (\text{S.3}) \end{aligned}$$

Let  $E_{0,X} = \mathbf{E}(R_0 - S_0X \mid X)$  and  $\ell$  be the largest integer strictly less than  $\nu$ . By Taylor expansion,

$$\begin{aligned} E_{0,X} &= \mathbf{E} \left[ \frac{1}{mh} \sum_{j=1}^m K \left( \frac{T_j - t}{h} \right) \{X(T_j) + \zeta_j - X(t)\} \mid X \right] \\ &= \frac{1}{mh} \sum_{j=1}^m \mathbf{E} \left[ K \left( \frac{T_j - t}{h} \right) \left\{ \frac{X^{(\ell)}(t + \tau_j(T_j - t)) - X^{(\ell)}(t)}{\ell!} (T_j - t)^\ell \right\} \mid X \right], \end{aligned}$$

where  $\tau_j \in [0, 1]$ . Hence, with  $u_\nu$  denoting  $\int_{-1}^1 K(s) |s|^\nu ds$ ,

$$\begin{aligned} |E_{0,X}| &\leq \frac{1}{mh} \sum_{j=1}^m \mathbf{E} \left\{ K \left( \frac{T_j - t}{h} \right) \left| \frac{X^{(\ell)}(t + \tau_j(T_j - t)) - X^{(\ell)}(t)}{\ell!} (T_j - t)^\ell \right| \mid X \right\}, \\ &\leq \frac{1}{h\ell!} L_X \mathbf{E} \left\{ K \left( \frac{T - t}{h} \right) |T - t|^\nu \right\} \leq \frac{L_X C_{T,2}}{\ell!} h^\nu u_\nu. \end{aligned} \quad (\text{S.4})$$

Let  $\sigma_{r,X} = \mathbf{E} \left( [h^{-1} K \{(T_j - t)/h\} \{X(T_j) + \zeta_j - X(t)\} - E_{0,X}]^r \mid X \right)$ . Then, for  $r \geq 2$ ,

$$\begin{aligned} \sigma_{r,X} &= \mathbf{E} \left( \left[ \frac{1}{h} K \left( \frac{T_j - t}{h} \right) \{X(T_j) + \zeta_j - X(t)\} - E_{0,X} \right]^r \mid X \right) \\ &\leq 3^r \mathbf{E} \left[ \left\{ \frac{1}{h} K \left( \frac{T_j - t}{h} \right) |X(T_j) - X(t)| \right\}^r \mid X \right] + 3^r \mathbf{E} \left[ \left\{ \frac{1}{h} K \left( \frac{T_j - t}{h} \right) |\zeta_j| \right\}^r \mid X \right] + 3^r |E_{0,X}|^r \\ &\leq 2 \cdot 3^r \left\{ \sup_t |X(t)|^r \right\} \mathbf{E} \left[ \left\{ \frac{1}{h} K \left( \frac{T_j - t}{h} \right) \right\}^r \right] + 3^r \mathbf{E} \left[ \left\{ \frac{1}{h} K \left( \frac{T_j - t}{h} \right) \right\}^r |\zeta_j|^r \right] + 3^r |E_{0,X}|^r \\ &\leq 2 \cdot 3^r \left\{ \sup_t |X(t)|^r \right\} h^{1-r} C_{T,2}^r + 3^r h^{1-r} C_{T,2}^r \mathbf{E} |\zeta|^r + 3^r L_X^r C_{T,2}^r h^{r\nu} u_\nu^r. \end{aligned} \quad (\text{S.5})$$

With (S.4) and (S.5), by Lemma S.2, conditioning on  $X$ , we have  $\mathbf{E} \{(R_0 - S_0X - E_{0,X})^{4p} \mid X\} \leq c_1(p) C_{T,2}^{4p} \{\sup_t |X(t)|^{4p} + L_X^{4p} u_\nu^{4p}\} m^{-2p} h^{-2p}$ , where  $c_j(p)$  denote a constant depending on  $p$  only for any  $j$ . This implies that

$$\begin{aligned} \mathbf{E} \{(R_0 - S_0X)^{4p} \mid X\} &\leq 2^{4p} \mathbf{E} \{(R_0 - S_0X - E_{0,X})^{4p} \mid X\} + 2^{4p} \mathbf{E} \{(E_{0,X})^{4p} \mid X\} \\ &\leq 2^{4p} c_1(p) C_{T,2}^{4p} \{\sup_t |X(t)|^{4p} + L_X^{4p} u_\nu^{4p}\} m^{-2p} h^{-2p} + (2C_{T,2} u_\nu)^{4p} h^{4p\nu} L_X^{4p}. \end{aligned} \quad (\text{S.6})$$

By a similar argument, we can show that  $\mathbf{E}(S_2 - \mathbf{E}S_2)^{4p} \leq c_2(p)m^{-2p}h^{-2p}$ . Also, it is easy to check that  $C_{T,1}u_2 \leq \mathbf{E}S_2 \leq C_{T,2}u_2$  with  $u_q$  denoting  $\int_{-1}^1 K(u)|u|^q du$  and hence

$$\mathbf{E}(S_2^{4p}) \leq 2^{4p}\mathbf{E}(S_2 - \mathbf{E}S_2)^{4p} + 2^{4p}|\mathbf{E}S_2|^{4p} \leq C_{T,2}^{4p}u_2^{4p} + c_2(p)m^{-2p}h^{-2p} = O(1). \quad (\text{S.7})$$

The same argument leads to  $\mathbf{E}\{S_0S_2 - S_1^2 - \mathbf{E}(S_0S_2 - S_1^2)\}^{2p} \leq c_3(p)m^{-p}h^{-p}$ . Note that  $\inf_t \mathbf{E}(S_0S_2 - S_1^2) > 0$  so that  $\{\mathbf{E}(S_0S_2 - S_1^2)\}^{-1} = O(1)$ . By Lemma S.3, this also implies that

$$\int_D \mathbf{E} \left\{ \left( \frac{1}{S_0S_2 - S_1^2 + \Delta} \right)^{2p} \right\} dt = O(1) + O(m^{-p}h^{-p} + m^{-4p}) = O(1). \quad (\text{S.8})$$

Putting (S.3), (S.6), (S.7) and (S.8) together, we conclude that

$$\mathbf{E}(\|I_1\|^p \mid X) = c_4(p) \left[ \left\{ \sup_t |X(t)|^p + L_X^p \right\} m^{-p/2} h^{-p/2} + h^{p\nu} L_X^p \right]. \quad (\text{S.9})$$

The same rate for  $I_2$  can be obtained in a similar fashion. For  $I_3$ , we have

$$\|I_3\|^p = \left\{ \int_D \left( \frac{\Delta X}{S_0S_2 - S_1^2 + \Delta} \right)^2 dt \right\}^{p/2} \leq \Delta^p \sup_t |X(t)|^p \left\{ \int_D \left( \frac{1}{S_0S_2 - S_1^2 + \Delta} \right)^2 dt \right\}^{p/2}.$$

Therefore, with (S.8),

$$\mathbf{E}(\|I_3\|^p \mid X) \leq \Delta^p \sup_t |X(t)|^p \int_D \mathbf{E} \left\{ \left( \frac{1}{S_0S_2 - S_1^2 + \Delta} \right)^{2p} \right\} dt \leq O(m^{-2p}) \sup_t |X(t)|^p. \quad (\text{S.10})$$

Now, by (S.9) and (S.10), observing that  $m^{-2p}$  is asymptotically dominated by  $m^{-p/2}h^{-p/2}$ , with (S.2) we conclude that

$$\mathbf{E}(\|\hat{X} - X\|^p \mid X) = O(m^{-p/2}h^{-p/2}) \left\{ \sup_t |X(t)|^p + L_X^p \right\} + O(h^{p\nu}) L_X^p. \quad (\text{S.11})$$

Then the statement (S.1) follows from  $p \geq 1$ .  $\square$

**Lemma S.2.** *Suppose  $V_1, V_2, \dots, V_N$  are i.i.d. random variables with mean zero. Assume  $\mathbf{E}V^r \leq a^r h^{1-r} + b^r h^{\kappa r}$  for some constants  $a, b, \kappa \geq 0$  and  $r \geq 2$ . Suppose  $h \geq N^{-1}$ . Then, for any integer  $p \geq 1$ , we have*

$$\mathbf{E} \left\{ \left( \frac{1}{N} \sum_{j=1}^N V_j \right)^{2p} \right\} \leq (2p)^{p-1} (2p)! p 2^p (a^{2p} + b^{2p}) N^{-p} h^{-p}.$$

PROOF. By multinomial theorem,

$$\left( \sum_{j=1}^N V_j \right)^{2p} = \sum_{k_1 + \dots + k_N = 2p} \binom{2p}{k_1, k_2, \dots, k_N} \prod_{j=1}^N V_j^{k_j}.$$

For each  $\prod_{j=1}^N V_j^{k_j}$ , if  $k_j = 1$  for some  $j$ , then it is zero. Let  $S(k_1, \dots, k_N)$  denote the number of non-zero  $k_j$ . Then, there are in total  $\binom{N}{1}$  items such that  $S(k_1, \dots, k_N) = 1$ , at most  $\binom{N}{2} (2p)$  items such that  $S(k_1, \dots, k_N) = 2$ , etc. In fact, there are at most  $\binom{N}{q} (2p)^{q-1}$  items such that  $S(k_1, \dots, k_N) = q$ , for every  $q \leq p$ . Note that by assumption,  $\mathbf{E}V^r \leq a^r h^{1-r} + b^r h^{\nu \kappa r} \leq (a^r + b^r) h^{1-r}$  for  $r \geq 2$ . Therefore,

$$\begin{aligned} \mathbf{E} \left( \sum_{j=1}^N V_j \right)^{2p} &\leq \sum_{q=1}^p \binom{N}{q} (2p)^{q-1} \binom{2p}{k_1, k_2, \dots, k_N} 2^q (a^{2p} h^{q-2p} + b^{2p} h^{q-2p}) \\ &\leq (2p)^{p-1} (2p)! 2^p (a^{2p} + b^{2p}) \sum_{q=1}^p \frac{N!}{(N-q)! q!} h^{q-2p} \\ &\leq (2p)^{p-1} (2p)! p 2^p (a^{2p} + b^{2p}) \sum_{q=1}^p N^p h^{q-2p} \\ &\leq (2p)^{p-1} (2p)! p 2^p (a^{2p} + b^{2p}) N^p h^{-p}. \end{aligned}$$

Multiplying both sides by  $N^{-2p}$  yields the conclusion of the lemma.  $\square$

**Lemma S.3.** *Suppose  $D \subset \mathbb{R}^p$  is compact set and  $S_N(t)$  for  $t \in D$  is a sequence of random processes defined on  $D$ . For  $b_N > 0$ , define  $\delta_N(t) = 2b_N 1_{\{|S(t)| \leq b_N\}}$ . Suppose for some constant  $c_0$ ,*

$0 < c_0 \leq \mathbf{E}S_N(t) < \infty$  for all  $t$  and sufficiently large  $N$ . Also, assume  $\lim_{N \rightarrow \infty} \inf_{t \in D} \mathbf{E}S_N(t) > 0$ .

For a sequence of  $a_N \rightarrow 0$  and any  $p > 0$ , if  $b_N^{-r} a_N^p \leq 1$  for some  $p$  and  $r > 0$ , and

1. if  $\mathbf{E}(\sup_{t \in D} |S_N(t) - \mathbf{E}S(t)|^p) = O(a_N^p)$ , then we have

$$\mathbf{E} \sup_{t \in D} \left| \frac{1}{S_N(t) + \delta_N(t)} - \frac{1}{\mathbf{E}S_N(t)} \right|^r = O(a_N^r + b_N^r);$$

2. if  $\int_D \mathbf{E}(|S_N(t) - \mathbf{E}S_N(t)|^p) dt = O(a_N^p)$ , then we have

$$\mathbf{E} \int \left| \frac{\mathbf{E}S_N(t)}{S_N(t) + \delta_N(t)} - 1 \right|^r dt = O(a_N^r + b_N^r).$$

PROOF. From now on, we shall suppress  $N$  when there is no confusion raised. Let  $\tilde{S}(t) = S(t) + \delta(t)$  and  $v(t) = \mathbf{E}\tilde{S}(t) - \mathbf{E}\delta(t) = \mathbf{E}S(t)$ . For a fixed  $t$  that is suppressed below,

$$\begin{aligned} \left| \frac{v}{\tilde{S}} - 1 \right|^r &\leq \left( \frac{|\tilde{S} - v|^r}{|\tilde{S}|^r} \right) 1_{\{|\tilde{S} - v| \leq v/2\}} + \left( \frac{|\tilde{S} - v|^r}{|\tilde{S}|^r} \right) 1_{\{|\tilde{S} - v| > v/2\}} \\ &\leq (v/2)^{-r} |\tilde{S} - v|^r + b_N^{-r} |\tilde{S} - v|^r 1_{\{|\tilde{S} - v| > v/2\}} \\ &\leq c_r (v/2)^{-r} |S - \mathbf{E}S|^r + c_r (v/2)^{-r} \delta^r + b_N^{-r} |\tilde{S} - v|^r 1_{\{|\tilde{S} - v| > v/2\}} \\ &\equiv I_1 + I_2 + I_3, \end{aligned}$$

where  $c_r > 0$  is a constant independent of  $t$ .

(1) By assumption,  $\mathbf{E} \sup_t I_1 = O(a_N^r)$ . Since  $|\delta| \leq 2b_N$ , we have  $\mathbf{E} \sup_t I_2 = O(b_N^r)$ . Also,

$$\mathbf{E} \sup_t I_3 \leq c_p b_N^{-r} \sup_t (v/2)^{-p} \mathbf{E}(\sup_t |S - v|^{p+r} + \sup_t |\delta|^{p+r}) = O(b_N^{-r} a_N^{p+r}) = O(a_N^r + b_N^r)$$

for sufficiently large  $p$ , and a constant  $c_p > 0$ .

(2) By assumption,  $\int I_1 dt = O(a_N^r)$ . Since  $|\delta| \leq 2b_N$ , we have  $\int I_2 dt = O(b_N^r)$ . Also,

$$\int I_3 dt \leq b_N^{-r} \int \{v(t)/2\}^{-p} \mathbf{E} |\tilde{S}(t) - v(t)|^{p+r} dt = O(b_N^{-r} a_N^{p+r}) = O(a_N^r + b_N^r).$$

Therefore, the conclusion of part (2) follows.  $\square$

In order to state the following lemmas, we shall first establish some notations and convention. Let  $u_{q,k} = \int_{\mathbb{B}_1(0)} K^q(\|u\|_{\mathbb{R}^d}) \|u\|_{\mathbb{R}^d}^k du$ . We also identify  $\iota_* T_x \mathcal{M}$  with  $\mathbb{R}^d$ . Let  $\mathbb{D}_{x,h}$  denote the set  $\{\theta \in \mathbb{R}^d : \exp_x(\theta) \in \mathbb{B}_h^{\mathcal{M}}(x)\}$ , where  $\exp_x$  denotes the exponential map at  $x$ . Let  $\kappa_{11,q} = \int_{h^{-1}\mathbb{D}_{x,h}} K^q(\|u\|_{\mathbb{R}^d}) du$ ,  $\kappa_{12,q,j} = \int_{h^{-1}\mathbb{D}_{x,h}} K^q(\|u\|_{\mathbb{R}^d}) \theta_j du$  and  $\kappa_{22,q,j,k} = \int_{h^{-1}\mathbb{D}_x} K^q(h^{-1}\|\theta\|_{\mathbb{R}^d}) \theta_j \theta_k d\theta$ , where  $\theta_j$  denotes the  $j$ th component of  $\theta$ . Let  $\pi_{d-1}$  denote the volume of the unit sphere  $S^{d-1}$ . The following three lemmas are based on Lemma A.2.5 of Cheng and Wu (2013) and hence their proofs are omitted.

**Lemma S.4.** *Suppose  $K$  is a kernel function compactly supported in  $[-1, 1]$  and continuously differentiable in  $[0, 1]$ . Let  $h \geq h_{pca}$ .*

1. *If  $x \in \mathcal{M} \setminus \mathcal{M}_h$ , then*

$$n^{-1} \sum_{i=1}^n h^{-d} K^q \left( \frac{\|X_i - x\|_{\mathcal{L}^2}}{h} \right) = u_{q,0} f(x) + O(h^2) + O_P(n^{-\frac{1}{2}} h^{-\frac{d}{2}})$$

2. *If  $x \in \mathcal{M}_h$ , then*

$$n^{-1} \sum_{i=1}^n h^{-d} K^q \left( \frac{\|X_i - x\|_{\mathcal{L}^2}}{h} \right) = f(x) \kappa_{11,q} + O(h) + O_P(n^{-\frac{1}{2}} h^{-\frac{d}{2}}).$$

**Lemma S.5.** *Suppose  $K$  is a kernel function compactly supported in  $[-1, 1]$  and continuously differentiable in  $[0, 1]$ . Let  $h \geq h_{pca}$  and  $\hat{\varphi}_k$  be the estimate in Theorem 1. Then,*

1. if  $x \in \mathcal{M} \setminus \mathcal{M}_h$ ,

$$\begin{aligned} & \frac{1}{n} \sum_{i=1}^n h^{-d} K^q \left( \frac{\|X_i - x\|_{\mathcal{L}^2}}{h} \right) \langle X_i - x, \hat{\varphi}_k \rangle \\ &= h^2 u_{q,1} d^{-1} \nabla_{\phi_k} f(x) + O_P(h^3 + n^{-\frac{1}{2}} h^{-\frac{d}{2}+1} + h^2 h_{pca}^{3/2} + h^3 h_{pca}). \end{aligned}$$

2. if  $x \in \mathcal{M}_h$ ,

$$\frac{1}{n} \sum_{i=1}^n h^{-d} K^q \left( \frac{\|X_i - x\|_{\mathcal{L}^2}}{h} \right) \langle X_i - x, \hat{\varphi}_k \rangle = h \kappa_{12,q,k}(x) + O_P(h^2 + n^{-\frac{1}{2}} h^{-\frac{d}{2}+1} + h h_{pca}^{3/2} + h^2 h_{pca}).$$

**Lemma S.6.** Suppose  $K$  is a kernel function compactly supported in  $[-1, 1]$  and continuously differentiable in  $[0, 1]$ . Let  $h \geq h_{pca}$ .

1. If  $x \in \mathcal{M} \setminus \mathcal{M}_h$ , then

$$\begin{aligned} & n^{-1} \sum_{i=1}^n h^{-d} K^q \left( \frac{\|X_i - x\|_{\mathcal{L}^2}}{h} \right) \langle X_i - x, \hat{\varphi}_j \rangle \langle X_i - x, \hat{\varphi}_k \rangle \\ &= \begin{cases} h^2 u_{q,2} d^{-1} f(x) + O_P(h^{\frac{7}{2}} + n^{-\frac{1}{2}} h^{-\frac{d}{2}+2}) & \text{if } 1 \leq j = k \leq d \\ O_P(h^{\frac{7}{2}} + n^{-\frac{1}{2}} h^{-\frac{d}{2}+2}) & \text{otherwise.} \end{cases} \end{aligned}$$

2. If  $x \in \mathcal{M}_h$ , then

$$\begin{aligned} & n^{-1} \sum_{i=1}^n h^{-d} K^q \left( \frac{\|X_i - x\|_{\mathcal{L}^2}}{h} \right) \langle X_i - x, \hat{\varphi}_j \rangle \langle X_i - x, \hat{\varphi}_k \rangle \\ &= h^2 f(x) \kappa_{22,q,j,k}(x) + O_P(h^3 + n^{-\frac{1}{2}} h^{-\frac{d}{2}+2} + h^2 h_{pca}^{3/2}). \end{aligned}$$

In order to prove Theorem 1, we establish the following auxiliary lemmas.

**Lemma S.7.** *Let  $\tilde{G} = \hat{G} + \Delta$  with  $\Delta = 1/\log n$ . Then  $\mathbf{E}|\log \tilde{G} - \log G| = o(1)$ . This result also holds for  $\hat{\mathcal{C}}_{\tilde{x}}$ , if  $\tilde{x}$  is independent of  $\hat{X}_1, \dots, \hat{X}_n$ , and that  $\{\mathbf{E}\|\tilde{x} - x\|^p\}^{1/p} = O(n^{-\beta})$  for all  $p \geq 1$ .*

*Proof.* By Jensen's inequality and concavity of  $\log(\cdot)$ ,

$$\begin{aligned} \mathbf{E}(\log \tilde{G} - \log G) &\leq \log \mathbf{E} \frac{\tilde{G}}{G} = \log \mathbf{E} \frac{\|X - x\|}{\|\hat{X} - x\| + \Delta} \leq \log \mathbf{E} \frac{\|\hat{X} - x\| + \|\hat{X} - X\|}{\|\hat{X} - x\| + \Delta} \\ &\leq \log(1 + \Delta^{-1} \mathbf{E}\|\hat{X} - X\|) \equiv a_n \end{aligned}$$

with  $a_n \geq 0$  and  $a_n \rightarrow 0$ . For other other direction, we first observe that

$$\begin{aligned} \mathbf{E} \left( \frac{\tilde{G}}{G} \right)^{1/4} &= \mathbf{E} \left\{ \frac{1}{G^{1/4}} \mathbf{E}(\tilde{G}^{1/4} \mid X) \right\} \leq \mathbf{E} \left\{ \frac{1}{G^{1/4}} \mathbf{E}(\|\hat{X} - X\|^{1/4} + \|X - x\|^{1/4} + \Delta^{1/4} \mid X) \right\} \\ &\leq \mathbf{E} \left[ \frac{C_1^{1/4} n^{-\beta/4} \{\eta(X)\}^{1/4} + \Delta^{1/4} + G^{1/4}}{G^{1/4}} \right] \\ &\leq 1 + \left( \mathbf{E} G^{-1/2} \mathbf{E} \left[ C_1^{1/4} n^{-\beta/4} \{\eta(X)\}^{1/4} + \Delta^{1/4} \right]^2 \right)^{1/2} \\ &\leq 1 + \left( \mathbf{E} G^{-1/2} \right)^{1/2} 2^{1/2} \left( \mathbf{E} \left[ C_1^{1/2} n^{-\beta/2} \{\eta(X)\}^{1/2} + \Delta^{1/2} \right] \right)^{1/2} \\ &\leq 1 + O(n^{-\beta/4} + (\log n)^{-1/4}) \end{aligned}$$

where  $C_1 > 0$  is some constant. This implies that

$$\frac{1}{4} \mathbf{E}(\log G - \log \tilde{G}) = \mathbf{E} \log \left( \frac{\tilde{G}}{G} \right)^{1/4} \leq \log \mathbf{E} \left( \frac{\tilde{G}}{G} \right)^{1/4} \equiv \frac{b_n}{4}$$

with  $b_n \geq 0$  and  $b_n \rightarrow 0$ , or equivalently,

$$\mathbf{E}(\log \tilde{G} - \log G) \geq -b_n.$$

Therefore  $\mathbf{E}|\log \tilde{G} - \log G| \leq a_n + b_n = o(1)$ . Following almost the same lines, we can deduce the

same result for  $\tilde{G}(\tilde{x})$ , i.e., the quantity  $\tilde{G}(x)$  when  $x$  is replaced with  $\tilde{x}$ .  $\square$

**Lemma S.8.** *Let  $\tilde{x}$  be an estimate of  $x$  such that  $\tilde{x}$  is independent of  $X$  and  $\hat{X}$ , and that  $\{\mathbf{E}\|\tilde{x} - x\|^p\}^{1/p} = O(n^{-\beta})$  for all  $p \geq 1$ . Suppose  $0 < a < \beta$ ,  $h \asymp n^{-a}$  and  $h_+ = h + n^{-(\beta+a)/2}$ . Let  $\tilde{Z} = 1_{\{\hat{X} \in \mathbb{B}_h^{\mathcal{L}^2}(\tilde{x})\}}$  and  $V = 1_{\{X \in \mathbb{B}_{h_+}^{\mathcal{L}^2}(x)\}}$ . If  $F$  is a positive functional of  $X$  and  $\hat{X}$  such that  $\mathbf{E}\{F(X, \hat{X})V\} = O(h^b)$  for some  $b \geq 0$ , and  $\mathbf{E}\{F(X, \hat{X})\}^q < \infty$  for some  $q > 1$ , then we have  $\mathbf{E}\{F(X, \hat{X})|\tilde{Z} - V|\} = O(h^b)$  and  $\mathbf{E}\{F(X, \hat{X})\tilde{Z}\} = O(h^b)$ . Also,  $\mathbf{E}\{F(X, \hat{X})|Z - \tilde{Z}|\} = o(h^b)$  with  $Z$  denoting  $1_{\{\hat{X} \in \mathbb{B}_h^{\mathcal{L}^2}(x)\}}$*

PROOF. Let  $\kappa = n^{-(\beta+a)/2}$  and  $\tilde{V} = 1_{\{X \in \mathbb{B}_{h_+}^{\mathcal{L}^2}(\tilde{x})\}}$ . Choose  $r > 1$  such that  $r^{-1} + q^{-1} = 1$ . To reduce notational burden, we simply use  $F$  to denote  $F(X, \hat{X})$ .

We shall first establish that  $\mathbf{E}(F|V - \tilde{V}|) = O(h^b)$ . To this end, we observe that

$$\mathbf{E}(F|V - \tilde{V}|) \leq \mathbf{E}(FV1_{\tilde{V}=0}) + \mathbf{E}(F\tilde{V}1_{V=0}).$$

For the first term, for any fixed  $s \geq 2rab/(\beta - a)$ , we have

$$\begin{aligned} \mathbf{E}(FV1_{\tilde{V}=0}) &= \mathbf{E}\{F1_{\|X-x\| \leq h, \|X-\tilde{x}\| \geq h}\} \\ &\leq \mathbf{E}\{F1_{\|\tilde{x}-x\| \geq \kappa, \|X-x\| \leq h} + F1_{h-\kappa \leq \|X-x\| \leq h}\} \\ &\leq \mathbf{E}\{F1_{\|\tilde{x}-x\| \geq \kappa}\} + \mathbf{E}\{FV\} \\ &\leq \{\mathbf{E}F^q\}^{1/q} \Pr(\|\tilde{x} - x\| \geq \kappa)^{1/r} + O(h^b) \\ &\leq \{\mathbf{E}F^q\}^{1/q} \left(n^{s(\beta+a)/2} \mathbf{E}\|\tilde{x} - x\|^s\right)^{1/r} + O(h^b) \\ &= O(n^{s(\beta+a)/(2r)-s\beta/r} + h^b) = O(h^b). \end{aligned}$$

Similar result can be derived for the second term. Thus, we prove that  $\mathbf{E}(F|V - \tilde{V}|) = O(h^b)$ .

Define  $h_- = h - \kappa$ ,  $\tilde{U} = 1_{\{X \in \mathbb{B}_{h_-}^{\mathcal{C}^2}(\tilde{x})\}}$ . Note that  $\tilde{U} \leq \tilde{V}$ . Then, by Hölder inequality, we have

$$\begin{aligned}
\mathbf{E}(F|\tilde{Z} - \tilde{V}|) &= \mathbf{E}(F1_{\tilde{Z}=1}1_{\tilde{V}=0}) + \mathbf{E}(F1_{\tilde{Z}=0}1_{\tilde{V}=1}) + \mathbf{E}(F1_{\tilde{Z}=0}1_{\tilde{V}=1}1_{\tilde{U}=0}) \\
&\leq \mathbf{E}(F1_{\tilde{Z}=1}1_{\tilde{V}=0}) + \mathbf{E}(F1_{\tilde{Z}=0}1_{\tilde{V}=1}) + \mathbf{E}(F\tilde{V}1_{\tilde{U}=0}) \\
&\leq (\mathbf{E}F^q)^{1/q} \left\{ (\mathbf{E}1_{\tilde{Z}=1}1_{\tilde{V}=0})^{1/r} + (\mathbf{E}1_{\tilde{Z}=0}1_{\tilde{V}=1})^{1/r} \right\} + O(h^b) \\
&\leq 2(\mathbf{E}F^q)^{1/q} \{ \Pr(\|X - \hat{X}\| \geq n^{-(\beta+a)/2}) \}^{1/r} + O(h^b) \\
&\leq 2(\mathbf{E}F^q)^{1/q} \left( n^{s(\beta+a)/2} \mathbf{E}\|X - \hat{X}\|^s \right)^{1/r} + O(h^b) \\
&= O\left( n^{s(\beta+a)/(2r) - s\beta/r} \right) + O(h^b) = O(h^b).
\end{aligned}$$

Then  $\mathbf{E}(F|\tilde{Z} - V|) \leq \mathbf{E}(F|\tilde{Z} - \tilde{V}|) + \mathbf{E}(F|\tilde{V} - V|) = O(h^b)$ . Since  $|\mathbf{E}(F\tilde{Z}) - \mathbf{E}(FV)| \leq \mathbf{E}(F|\tilde{Z} - V|)$ , the result  $\mathbf{E}(F\tilde{Z}) = O(h^b)$  follows.  $\square$

**Lemma S.9.** Suppose  $\{\psi_k\}_{k=1}^\infty$  is an orthonormal basis of  $\mathcal{H}$  and  $x \in \mathcal{M}$  is fixed. Assume that  $\{\psi_1, \dots, \psi_d\}$  span the tangent space  $\iota_* T_x \mathcal{M}$ . Let  $\pi_{d-1}$  be the volume of the  $d-1$  dimensional unit sphere  $S^{d-1}$  and  $\hat{\mathcal{C}}_x$  the sample covariance operator based on  $\hat{\mathcal{N}}_{\mathcal{L}^2}(h, x)$  for some  $h \asymp n^{-a}$  with  $0 < a < \beta$ . Then,

$$\begin{aligned}
\sup_{j \leq d} \sup_{k \geq d+1} |\langle \hat{\mathcal{C}}_x \psi_j, \psi_k \rangle| &= O_P \left( h^{d+4} \log n + n^{-1/2} h^{d/2+3} + n^{-\beta} h^{d+1} \right), \\
\sup_{j, k \geq d+1} |\langle \hat{\mathcal{C}}_x \psi_j, \psi_k \rangle| &= O_P \left( h^{d+4} + n^{-1/2} h^{d/2+4} + n^{-\beta} h^{d+1} \right), \\
\sup_{1 \leq j \neq k \leq d} |\langle \hat{\mathcal{C}}_x \psi_j, \psi_k \rangle| &= O_P \left( h^{d+3} + n^{-1/2} h^{d/2+3} + n^{-\beta} h^{d+1} \right), \\
\text{for } 1 \leq k \leq d: \quad \langle \hat{\mathcal{C}}_x \psi_k, \psi_k \rangle &= \pi_{d-1} f(x) d^{-1} h^{d+2} + O_P \left( n^{-1/2} h^{d/2+2} + n^{-\beta} h^{d+1} \right).
\end{aligned}$$

The above results hold also for  $\hat{\mathcal{C}}_{\tilde{x}}$ , if  $\tilde{x}$  is independent of  $\hat{X}_1, \dots, \hat{X}_n$ , and that  $\{\mathbf{E}\|\tilde{x} - x\|^p\}^{1/p} = O(n^{-\beta})$  for all  $p \geq 1$ .

PROOF. Denote  $Z_i = 1_{\{\hat{X}_i \in \mathbb{B}_h^{\mathcal{C}^2}(x)\}}$ . Then  $\hat{\mathcal{C}}_x$  can be written as  $\hat{\mathcal{C}}_x = n^{-1} \sum_{i=1}^n (\hat{X}_i - \hat{\mu}_x) \otimes (\hat{X}_i - \hat{\mu}_x) Z_i$ ,

where  $\hat{\mu}_x = \sum_{i=1}^n \hat{X}_i Z_i$ . For any  $y, z$  such that  $\|y\|_{\mathcal{L}^2} = \|z\|_{\mathcal{L}^2} = 1$ , we have

$$\begin{aligned}
\langle \hat{\mathcal{C}}_x y, z \rangle &= \langle n^{-1} \sum_{i=1}^n Z_i (\hat{X}_i - \hat{\mu}_x) \otimes (\hat{X}_i - \hat{\mu}_x) y, z \rangle = n^{-1} \sum_{i=1}^n \langle \hat{X}_i - \hat{\mu}_x, y \rangle \langle \hat{X}_i - \hat{\mu}_x, z \rangle Z_i \\
&= n^{-1} \sum_{i=1}^n \langle X_i - \mu_x, y \rangle \langle X_i - \mu_x, z \rangle Z_i + n^{-1} \sum_{i=1}^n \langle (\hat{X}_i - X_i) - (\hat{\mu}_x - \mu_x), y \rangle \langle \hat{X}_i - \hat{\mu}_x, z \rangle Z_i \\
&\quad + n^{-1} \sum_{i=1}^n \langle \hat{X}_i - \hat{\mu}_x, y \rangle \langle (\hat{X}_i - X_i) - (\hat{\mu}_x - \mu_x), z \rangle Z_i \\
&\quad + n^{-1} \sum_{i=1}^n \langle (\hat{X}_i - X_i) - (\hat{\mu}_x - \mu_x), y \rangle \langle (\hat{X}_i - X_i) - (\hat{\mu}_x - \mu_x), z \rangle Z_i \\
&\equiv I_1 + I_2 + I_3 + I_4,
\end{aligned}$$

where  $\mu_x = \sum_{i=1}^n X_i Z_i$ . Before we proceed to analyze  $I_1, I_2, I_3$  and  $I_4$ , we prepare some calculations.

First, it is easy to check that

$$\|\hat{\mu}_x - \mu_x\| = \left\| \frac{1}{n} \sum_{i=1}^n \{(X_i - \mu_x) + (\hat{X}_i - X_i)\} Z_i \right\| \leq \frac{1}{n} \sum_{i=1}^n \|\hat{X}_i - X_i\| Z_i.$$

This implies that

$$\sum_{i=1}^n \|\hat{\mu}_x - \mu_x\| Z_i \leq \sum_{i=1}^n \|\hat{\mu}_x - \mu_x\| \leq \sum_{i=1}^n \|\hat{X}_i - X_i\| Z_i \quad (\text{S.12})$$

and

$$\sum_{i=1}^n \|\hat{\mu}_x - \mu_x\|^2 Z_i \leq \sum_{i=1}^n \|\hat{\mu}_x - \mu_x\|^2 \leq 2 \sum_{i=1}^n \|\hat{X}_i - X_i\|^2 Z_i. \quad (\text{S.13})$$

Now we analyze  $I_2$ . It is seen that

$$\begin{aligned}
\mathbf{E} \sup_{y,z} |I_2| &\leq \mathbf{E} \sup_{y,z} \left| n^{-1} \sum_{i=1}^n \langle (\hat{X}_i - X_i) - (\hat{\mu}_x - \mu_x), y \rangle \langle \hat{X}_i - \hat{\mu}_x, z \rangle Z_i \right| \\
&\leq \mathbf{E} \sup_{y,z} n^{-1} \sum_{i=1}^n \|(\hat{X}_i - X_i) - (\hat{\mu}_x - \mu_x)\| \|\hat{X}_i - \hat{\mu}_x\| Z_i \\
&\leq \mathbf{E} \sup_{y,z} n^{-1} \sum_{i=1}^n \|(\hat{X}_i - X_i) - (\hat{\mu}_x - \mu_x)\| h Z_i \\
&\leq n^{-1} h \mathbf{E} \sum_{i=1}^n \left( \|\hat{X}_i - X_i\| + \|\hat{\mu}_x - \mu_x\| \right) Z_i \\
&\leq 2h \mathbf{E} \left( \|\hat{X}_i - X_i\| Z_i \right), \tag{S.14}
\end{aligned}$$

where the second inequality follows from Cauchy-Schwarz inequality and  $\|y\|_{\mathcal{L}^2} = \|z\|_{\mathcal{L}^2} = 1$ , the third one is from the fact that  $\hat{\mu}_x, \hat{X}_i \in \mathbb{B}_{\mathcal{L}_h^2}(x)$  for  $Z_i = 1$ , the fourth one follows from triangle inequality, the fifth inequality is based on (S.12). Now, let  $h_1 = h + n^{-(\beta+a)/2}$  and  $V_i = 1_{\{X_i \in \mathbb{B}_{h_1}^2(x)\}}$ . Based on assumption (B3),  $\mathbf{E}(\|\hat{X}_i - X_i\| V_i) = O(n^{-\beta} h_1^{d+1})$ . Then, by Lemma S.8,  $\mathbf{E}(\|\hat{X}_i - X_i\| Z_i) = O(n^{-\beta} h_1^{d+1}) = O(n^{-\beta} h^{d+1})$ , since  $h_1 \asymp h$ . With (S.14), this shows that  $\mathbf{E} \sup_{y,z} |I_2| = O(n^{-\beta} h^{d+1})$ . Similarly,  $\mathbf{E} \sup_{y,z} |I_3| = O(n^{-\beta} h^{d+1})$ .

For  $I_4$ , we have

$$\begin{aligned}
\mathbf{E} \sup_{y,z} |I_4| &= \mathbf{E} \sup_{y,z} n^{-1} \left| \sum_{i=1}^n \langle (\hat{X}_i - X_i) - (\hat{\mu}_x - \mu_x), y \rangle \langle (\hat{X}_i - X_i) - (\hat{\mu}_x - \mu_x), z \rangle Z_i \right| \\
&\leq \mathbf{E} \sup_{y,z} n^{-1} \sum_{i=1}^n \|(\hat{X}_i - X_i) - (\hat{\mu}_x - \mu_x)\|^2 Z_i \leq 2\mathbf{E} n^{-1} \sum_{i=1}^n (\|\hat{X}_i - X_i\|^2 + \|\hat{\mu}_x - \mu_x\|^2) Z_i \\
&\leq 4\mathbf{E} n^{-1} \sum_{i=1}^n \|\hat{X}_i - X_i\|^2 Z_i = 4\mathbf{E}(\|\hat{X}_i - X_i\|^2 Z_i),
\end{aligned}$$

where the first inequality comes from Cauchy-Schwarz inequality and  $\|y\|_{\mathcal{L}^2} = \|z\|_{\mathcal{L}^2} = 1$ , the second one follows from triangle inequality, and the third one is based on (S.13). By Lemma S.8, we can

show that  $\mathbf{E}(\|\hat{X}_i - X_i\|^2 Z_i) = O(n^{-2\beta} h^d)$ .

The order of  $I_1$  is given in Lemma S.10. Therefore, results of the lemma follow. It is easy but somewhat tedious to check that the above derivation also holds for  $\tilde{x}$ .  $\square$

**Lemma S.10.** *For  $0 < a < \beta$ , let  $h \asymp n^{-a}$  and  $h_1 = h + n^{-(\beta+a)/2}$ . Denote  $Z_i = 1_{\{\hat{X}_i \in \mathbb{B}_h^{\mathcal{L}^2}(x)\}}$  and  $\Xi_{j,k} = n^{-1} \sum_{i=1}^n \langle X_i - \mu_x, \psi_j \rangle \langle X_i - \mu_x, \psi_k \rangle Z_i$ , where  $\{\psi_k\}$  are defined in Lemma S.9. Then, we have*

$$\mathbf{E} \sup_{j \leq d} \sup_{k \geq d+1} |\Xi_{j,k}| = O(h^{d+3}), \quad (\text{S.15})$$

$$\mathbf{E} \sup_{j,k \geq d+1} |\Xi_{j,k}| = O(h^{d+4}), \quad (\text{S.16})$$

$$\text{for } 1 \leq j \neq k \leq d : \quad \mathbf{E} \Xi_{j,k} = O(h^{d+3}), \quad (\text{S.17})$$

$$\text{for } 1 \leq k \leq d : \quad \mathbf{E} \Xi_{k,k} = O(h^{d+2}). \quad (\text{S.18})$$

Also,

$$\mathbf{Var} \left( \sup_{j \leq d} \sup_{k \geq d+1} |\Xi_{j,k}| \right) = O(n^{-1} h^{d+6}), \quad (\text{S.19})$$

$$\mathbf{Var} \left( \sup_{j,k \geq d+1} |\Xi_{j,k}| \right) = O(n^{-1} h^{d+8}),$$

$$\text{for } 1 \leq j \neq k \leq d : \quad \mathbf{Var} (|\Xi_{j,k}|) = O(n^{-1} h^{d+6}),$$

$$\text{for } 1 \leq k \leq d : \quad \mathbf{Var} (\Xi_{k,k}) = O(n^{-1} h^{d+4}).$$

**PROOF.** Let  $V_i = 1_{\{X_i \in \mathbb{B}_{h_1}^{\mathcal{L}^2}(x)\}}$ . Since  $h_1 \asymp h$ , we shall use them exchangeably when no confusion arises. Let  $\mathcal{P}_1$  be projection into  $\{\psi_1, \dots, \psi_d\}$  and  $\mathcal{P}_2$  be projection into  $\{\psi_{d+1}, \dots\}$ . First, for

$$1 \leq j \leq d,$$

$$\begin{aligned}
\mathbf{E} \sup_{k \geq d+1} |\Xi_{j,k}| &\leq \mathbf{E} \sup_{k \geq d+1} \left| n^{-1} \sum_{i=1}^n \langle X_i - \mu_x, \psi_j \rangle \langle X_i - \mu_x, \psi_k \rangle Z_i \right| \\
&\leq \mathbf{E} \sup_{k \geq d+1} \left| n^{-1} \sum_{i=1}^n \langle X_i, \psi_j \rangle \langle X_i, \psi_k \rangle Z_i \right| \\
&\quad + \mathbf{E} \sup_{k \geq d+1} \left| n^{-1} \sum_{i=1}^n \langle \mu_x, \psi_j \rangle \langle \mu_x, \psi_k \rangle Z_i \right| \\
&= c_1(I_1 + I_2).
\end{aligned} \tag{S.20}$$

It is easy to see that  $I_1$  is the dominant term, which we evaluate below (utilizing the fact that  $\Pi_x(\theta, \theta) \perp T_x \mathcal{M}$ ):

$$\begin{aligned}
I_1 &= \mathbf{E} \sup_{k \geq d+1} \left| n^{-1} \sum_{i=1}^n \langle X_i, \psi_j \rangle \langle X_i, \psi_k \rangle Z_i \right| \leq \frac{1}{n} \mathbf{E} \sum_{i=1}^n \sup_{k \geq d+1} |\langle X_i, \psi_j \rangle \langle X_i, \psi_k \rangle Z_i| \\
&= \mathbf{E} \sup_{k \geq d+1} |\langle X_i, \psi_j \rangle \langle X_i, \psi_k \rangle Z_i| = \mathbf{E} \sup_{k \geq d+1} |\langle X_i, \psi_j \rangle \langle \mathcal{P}_2 X_i, \psi_k \rangle Z_i|. \\
&\leq \mathbf{E} (|\langle X_i, \psi_j \rangle| \|\mathcal{P}_2 X_i\| |Z_i|).
\end{aligned} \tag{S.21}$$

Since by Lemma A.2.4 of Cheng and Wu (2013),

$$\begin{aligned}
&\mathbf{E} |\langle X_i, \psi_j \rangle \langle \mathcal{P}_2 X_i, \psi_k \rangle Z_i| \\
&\leq \int_{S^{d-1}} \int_0^{h_1} \langle t \nu_* \theta, \psi_j \rangle \|t^2 \Pi_x(\theta, \theta)\|_{\mathcal{L}^2} f(\exp(t\theta)) t^{d-1} dt d\theta + O(h^{d+5}) \\
&= O(h^{d+3}),
\end{aligned}$$

we can apply Lemma S.8 to conclude  $\mathbf{E} (|\langle X_i, \psi_j \rangle| \|\mathcal{P}_2 X_i\| |Z_i|) = O(h^{d+3})$ , and hence with (S.21), we assert that  $I_1 = O(h^{d+3})$ . This proves (S.15). The result (S.16) is obtained in a similar way.

For (S.17), by the same argument of obtaining (S.20), we can show that for  $1 \leq j \neq k \leq d$ ,  $\mathbf{E} \Xi_{j,k}$

is dominated by

$$\mathbf{E} n^{-1} \sum_{i=1}^n \langle X_i, \psi_j \rangle \langle X_i, \psi_k \rangle Z_i = \mathbf{E} \langle X_i, \psi_j \rangle \langle X_i, \psi_k \rangle Z_i.$$

Now, because

$$\begin{aligned} & \mathbf{E} \langle X_i, \psi_j \rangle \langle X_i, \psi_k \rangle V_i \\ &= \int_{S^{d-1}} \int_0^{h_1} \langle t\iota_*\theta, \psi_j \rangle \langle t\iota_*\theta, \psi_k \rangle [f(x) + t\nabla_\theta f(x)] t^{d-1} dt d\theta + O(h^{d+4}) \\ &= O(h^{d+3}), \end{aligned}$$

where the second equality is based on the fact that the second fundamental form is self-adjoint, by Lemma S.8, (S.17) follows. The result (S.18) is derived in a similar fashion.

Let  $\chi_{i,k} = n^{-1} \langle X_i, \psi_j \rangle \langle X_i, \psi_k \rangle Z_i$ . Then  $\Xi_{j,k} = \sum_{i=1}^n \chi_{i,k}$ . Then by Theorem 11.1 of Boucheron et al. (2016), we have

$$\mathbf{Var} \left( \sup_{k \geq d+1} \Xi_{j,k} \right) = \mathbf{Var} \left( \sup_{k \geq d+1} \sum_{i=1}^n \chi_{i,k} \right) \leq \sum_{i=1}^n \mathbf{E} \sup_{k \geq d+1} \chi_{i,k}^2 = n \mathbf{E} \sup_{k \geq d+1} \chi_{i,k}^2. \quad (\text{S.22})$$

The term  $\mathbf{E} \sup_{k \geq d+1} \chi_{i,k}^2$  can be computed as follows:

$$\begin{aligned} \mathbf{E} \sup_{k \geq d+1} \chi_{i,k}^2 &= \mathbf{E} \sup_{k \geq d+1} \left[ n^{-1} \langle X_i, \psi_j \rangle \langle \mathcal{P}_2 X_i, \psi_k \rangle Z_i \right]^2 \\ &\leq n^{-2} \mathbf{E} \sup_{k \geq d+1} \|X_i\|^2 \|\mathcal{P}_2 X_i\|^2 \|\psi_j\|^2 \|\psi_k\|^2 Z_i = n^{-2} \mathbf{E} \|X_i\|^2 \|\mathcal{P}_2 X_i\|^2 Z_i. \end{aligned}$$

Since

$$\mathbf{E} \|X_i\|^2 \|\mathcal{P}_2 X_i\|^2 V_i = \int_{S^{d-1}} \int_0^{h_1} \|t\iota_*\theta\|^2 \|t^2 \Pi_x(\theta, \theta)\|^2 f(\exp(t\theta)) t^{d-1} dt d\theta + O(h^{d+8}) = O(h^{d+6}),$$

we apply Lemma S.8 to conclude  $\mathbf{E}\|X_i\|^2\|\mathcal{P}_2 X_i\|^2 Z_i = O(h^{d+6})$ . Therefore,  $\mathbf{E} \sup_{k \geq d+1} \chi_{i,k}^2 = O(n^{-2}h^{d+6})$ . With (S.22), we show that

$$\mathbf{Var} \left( \sup_{k \geq d+1} \Xi_{j,k} \right) = O(n^{-1}h^{d+6}).$$

Other results are derived in the same way. □

### S.3 Proof of Theorem 3

PROOF OF THEOREM 3. The proof is similar to the proof for Theorem 2. Below we shall only discuss those that are different. Let  $h = h_{reg}$  to reduce notational burden.

$$\begin{aligned} \frac{1}{n} \mathbf{X}^T \mathbf{W} \mathbf{X} &= f(x) \mathbf{v} \kappa_1 \mathbf{v} \\ &+ \begin{bmatrix} O(h) + O_P(n^{-\frac{1}{2}}h^{-\frac{d}{2}}) & O(h^2) + O_P(n^{-\frac{1}{2}}h^{-\frac{d}{2}+1}) \\ O(h^2) + O_P(n^{-\frac{1}{2}}h^{-\frac{d}{2}+1}) & O(h^3) + O_P(n^{-\frac{1}{2}}h^{-\frac{d}{2}+2}) \end{bmatrix} \end{aligned}$$

where

$$\kappa_q = \begin{bmatrix} \kappa_{11,q} & \kappa_{12,q} \\ \kappa_{12,q}^T & \kappa_{22,q} \end{bmatrix}, \kappa_{22,q} = (\kappa_{22,q,j,k})_{j,k=1}^d, \mathbf{v} = \begin{bmatrix} 1 & 0 \\ 0 & h \mathbf{I}_d \end{bmatrix}.$$

Therefore,

$$\begin{aligned} \frac{1}{n} \hat{\mathbf{X}}^T \hat{\mathbf{W}} \hat{\mathbf{X}} &= f(x) \mathbf{v} \kappa_1 \mathbf{v} \\ &+ \begin{bmatrix} O(h) + O_P(n^{-\frac{1}{2}}h^{-\frac{d}{2}}) + O_P(h^{-1-\epsilon d}n^{-\beta}) & O(h^2) + O_P(n^{-\frac{1}{2}}h^{-\frac{d}{2}+1}) + O_P(h^{-1-\epsilon d}n^{-\beta}) \\ O(h^2) + O_P(n^{-\frac{1}{2}}h^{-\frac{d}{2}+1}) + O_P(h^{-1-\epsilon d}n^{-\beta}) & O(h^3) + O_P(n^{-\frac{1}{2}}h^{-\frac{d}{2}+2}) + O_P(h^{-1-\epsilon d}n^{-\beta}) \end{bmatrix}. \end{aligned}$$

and hence

$$\begin{aligned} \left(\frac{1}{n}\hat{\mathbf{X}}^T\hat{\mathbf{W}}\hat{\mathbf{X}}\right)^{-1} &= \mathbf{v}^{-1}\kappa_1^{-1}\mathbf{v}^{-1}/f(x) \\ &+ \begin{bmatrix} O_P(h + h^{-2-\epsilon d}n^{-\beta} + n^{-\frac{1}{2}}h^{-\frac{d}{2}}) & O_P(1 + h^{-4-\epsilon d}n^{-\beta} + n^{-\frac{1}{2}}h^{-\frac{d}{2}-1}) \\ O_P(1 + h^{-4-\epsilon d}n^{-\beta} + n^{-\frac{1}{2}}h^{-\frac{d}{2}-1}) & O_P(h^{-1} + h^{-5-\epsilon d}n^{-\beta} + n^{-\frac{1}{2}}h^{-\frac{d}{2}-2}) \end{bmatrix}. \end{aligned}$$

This implies that

$$\mathbf{e}_1^T(\hat{\mathbf{X}}^T\hat{\mathbf{W}}\hat{\mathbf{X}})^{-1}\hat{\mathbf{X}}^T\hat{\mathbf{W}}\left\{(\mathbf{X} - \hat{\mathbf{X}})\begin{bmatrix} g(x) \\ \nabla g(x) \end{bmatrix}\right\} = \mathbf{e}_1^T\begin{bmatrix} 1 & h^{-1} \\ h^{-1} & h^{-2} \end{bmatrix}O_P(h^{-1-\epsilon d}n^{-\beta})\mathbf{1}_{d \times 1} = O_P(h^{-1-\epsilon d}n^{-\beta}).$$

By Lemma (S.4), (S.5) and (S.6), one can show that

$$\frac{1}{n}\mathbf{X}^T\mathbf{W}\mathbf{H} = \begin{bmatrix} h^2 f(x) \int_{\frac{1}{h}\mathbb{D}_x} K(\|\theta\|_{\mathbb{R}^d}) \text{Hess } g(x) \theta d\theta + O_P(h^3 + n^{-1/2}h^{-d/2+2}) \\ h^3 f(x) \int_{\frac{1}{h}\mathbb{D}_x} K(\|\theta\|_{\mathbb{R}^d}) \theta^T \text{Hess } g(x) \theta d\theta + O_P(h^{7/2} + n^{-\frac{1}{2}}h^{-\frac{d}{2}+3}) \end{bmatrix},$$

and hence

$$\frac{1}{n}\hat{\mathbf{X}}^T\hat{\mathbf{W}}\mathbf{H} = \begin{bmatrix} h^2 f(x) \int_{\frac{1}{h}\mathbb{D}_x} K(\|\theta\|_{\mathbb{R}^d}) \text{Hess } g(x) \theta d\theta + O_P(h^3 + n^{-1/2}h^{-d/2+2} + h^{-1-\epsilon d}n^{-\beta}) \\ h^3 f(x) \int_{\frac{1}{h}\mathbb{D}_x} K(\|\theta\|_{\mathbb{R}^d}) \theta^T \text{Hess } g(x) \theta d\theta + O_P(h^{7/2} + n^{-\frac{1}{2}}h^{-\frac{d}{2}+3} + h^{-1-\epsilon d}n^{-\beta}) \end{bmatrix}.$$

Thus, with the choice of  $h$ , which implies that  $n^{-\frac{1}{2}}h^{-\frac{d}{2}} \ll 1$  and  $h^{-1-\epsilon d}n^{-\beta} \ll h^3$ ,

$$\begin{aligned} \mathbf{e}_1^T(\hat{\mathbf{X}}^T\hat{\mathbf{W}}\hat{\mathbf{X}})^{-1}\hat{\mathbf{X}}^T\hat{\mathbf{W}}\left\{\frac{1}{2}\mathbf{H}(x) + O_P(h^3)\right\} &= h^2 \frac{\text{tr}(\text{Hess } g(x)\boldsymbol{\kappa}_{22,1})}{2(\boldsymbol{\kappa}_{11,1} - \boldsymbol{\kappa}_{12,1}^T \boldsymbol{\kappa}_{22,1}^{-1} \boldsymbol{\kappa}_{12,1})} \\ &+ O_P(h^{5/2} + n^{-\frac{1}{2}}h^{-\frac{d}{2}+2} + h^{-2-\epsilon d}n^{-\beta}). \end{aligned}$$

Therefore, the conditional bias is

$$\mathbf{E}\{\hat{g}(x) - g(x) \mid \mathcal{D}\} = h^2 \frac{\text{tr}(\text{Hess}g(x)\boldsymbol{\kappa}_{22,1})}{2(\boldsymbol{\kappa}_{11,1} - \boldsymbol{\kappa}_{12,1}^T \boldsymbol{\kappa}_{22,1}^{-1} \boldsymbol{\kappa}_{12,1})} + O_P(h^{5/2} + n^{-\frac{1}{2}}h^{-\frac{d}{2}+2} + h^{-2-\epsilon d}n^{-\beta}).$$

For the conditional variance, by Lemma S.4, S.5 and S.6, we have

$$\frac{1}{n}\mathbf{X}^T\mathbf{W}\mathbf{W}\mathbf{X} = f(x)\mathbf{v}\kappa_2\mathbf{v}h^{-d} + h^{-d} \begin{bmatrix} O(h) + O_P(n^{-\frac{1}{2}}h^{-\frac{d}{2}}) & O_P(h^2 + n^{-\frac{1}{2}}h^{-\frac{d}{2}+1}) \\ O_P(h^2 + n^{-\frac{1}{2}}h^{-\frac{d}{2}+1}) & O_P(h^{\frac{5}{2}} + n^{-\frac{1}{2}}h^{-\frac{d}{2}+2}) \end{bmatrix}.$$

Thus,

$$\begin{aligned} & n^{-1}\sigma_\zeta^2\mathbf{e}_1^T(n^{-1}\hat{\mathbf{X}}^T\hat{\mathbf{W}}\hat{\mathbf{X}})^{-1}(n^{-1}\mathbf{X}^T\mathbf{W}\mathbf{W}\mathbf{X})(n^{-1}\hat{\mathbf{X}}^T\hat{\mathbf{W}}\hat{\mathbf{X}})^{-1}\mathbf{e}_1^T \\ &= \frac{1}{nh^d}\frac{\sigma_\varepsilon^2}{f(x)}\mathbf{e}_1^T\kappa_{22,1}^{-1}\kappa_{22,2}\kappa_{22,1}^{-1}\mathbf{e}_1 + O_P\left(n^{-1}h^{-d}(h^{\frac{1}{2}} + n^{-\beta}h^{-4-\epsilon d} + n^{-\frac{1}{2}}h^{-\frac{d}{2}})\right). \end{aligned} \quad (\text{S.23})$$

Also, similar to (25), we have

$$\begin{aligned} & n^{-1}\sigma_\zeta^2\mathbf{e}_1^T(n^{-1}\hat{\mathbf{X}}^T\hat{\mathbf{W}}\hat{\mathbf{X}})^{-1}\mathbf{1}_{(d+1)\times(d+1)}(n^{-1}\hat{\mathbf{X}}^T\hat{\mathbf{W}}\hat{\mathbf{X}})^{-1}\mathbf{e}_1^T O_P(h^{-d-1-\epsilon d}n^{-\beta}) \\ &= n^{-1}O_P(h^{-2} + n^{-\beta}h^{-5-\epsilon d} + n^{-\frac{1}{2}}h^{-\frac{d}{2}-2})O_P(h^{-d-1-\epsilon d}n^{-\beta}). \\ &= O_P\left(n^{-1}h^{-d}h^{-1-\epsilon d}n^{-\beta}(h^{-2} + n^{-\beta}h^{-5-\epsilon d} + n^{-\frac{1}{2}}h^{-\frac{d}{2}-2})\right). \end{aligned} \quad (\text{S.24})$$

With  $n^{-\beta}h^{-2-\epsilon d} \ll h^2$ , combining (22), (23), (S.23) and (S.24), we conclude that the conditional variance is

$$\mathbf{Var}\{\hat{g}(x) \mid \mathcal{D}\} = \frac{1}{nh^d}\frac{\sigma_\varepsilon^2}{f(x)}\mathbf{e}_1^T\kappa_{22,1}^{-1}\kappa_{22,2}\kappa_{22,1}^{-1}\mathbf{e}_1 + o_P(n^{-1}h^{-d}).$$

□

## References

- Boucheron, S., Lugosi, G., and Massart, P. (2016). *Concentration Inequalities: A Nonasymptotic Theory of Independence*. Oxford University Press, Oxford, United Kingdom.
- Cheng, M. and Wu, H. (2013). Local linear regression on manifolds and its geometric interpretation. *Journal of the American Statistical Association*, 108:1421–1434.
